# Supplementary material for: Smart sensing of the multifunctional properties of magnetron sputtered $MoS_2$ across the amorphous-crystalline transition
Source: arXiv:2312.10180 ancillary file (2023-12-19)
Supplement: Supplementary file 1 [file supp_1912.pdf]

**Supplementary Materials for  
Smart sensing of the multifunctional properties of  
magnetron sputtered MoS<sub>2</sub> across the  
amorphous-crystalline transition.**

Jose L. Ocana-Pujol<sup>1</sup>, Rebecca A. Gallivan<sup>1</sup>, Ramon Camilo Dominguez Ordonez<sup>1</sup>,  
Nikolaus Porenta<sup>1</sup>, Arnold Müller<sup>2</sup>, Christof Vockenhuber<sup>2</sup>,  
Ralph Spolenak<sup>1</sup>, and Henning Galinski<sup>1</sup>

<sup>1</sup>Laboratory for Nanometallurgy, ETH Zurich, Zürich, Switzerland

<sup>2</sup>Laboratory of Ion Beam Physics, ETH Zurich, Zürich, Switzerland

# 1 Stability of the metal-MoS<sub>2</sub> system upon annealing

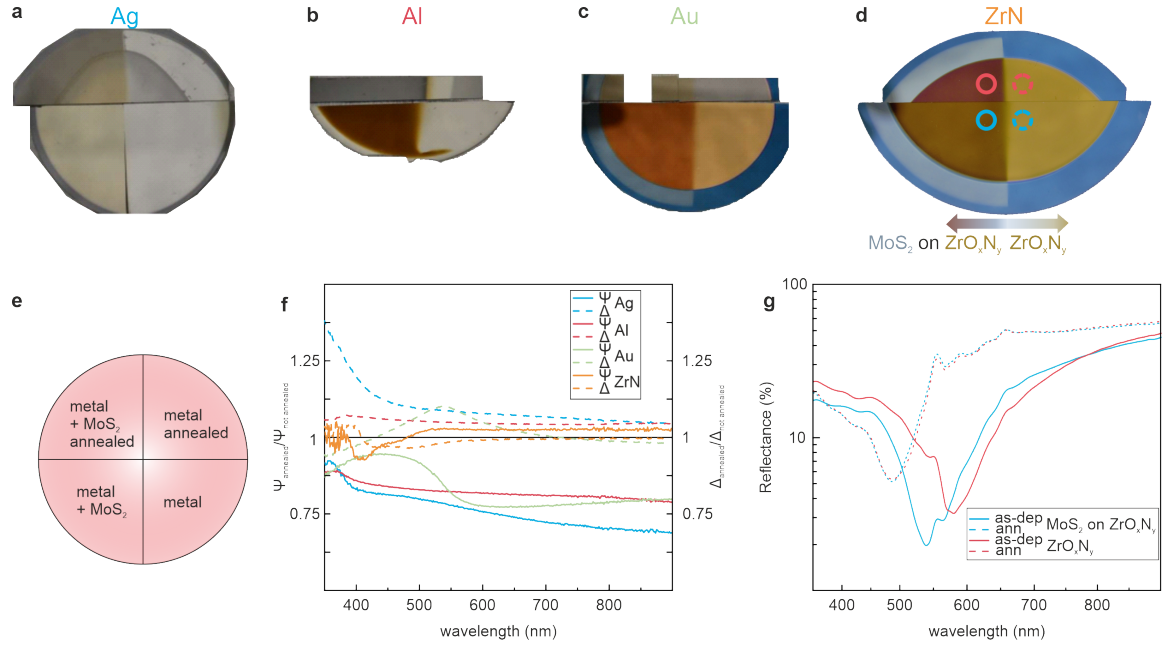

Figure S1: (a-d): Pictures of the wafers of sputtered metals with MoS<sub>2</sub> sputtered on the left side of the wafer. The bottom half of the picture is as-deposited, while the upper half is after annealing in UHV at 485°C. The metals are (a) silver , (b) aluminium, (c) gold, and (d) zirconium nitride. (e): Schematic explaining pictures (a)-(d). (f): Change in the ellipsometric properties of the sputtered metals upon annealing. (g): Reflectance of the different parts of the wafer with ZrN.

Figure S1 shows that ZrN is the MoS<sub>2</sub> coated substrate that has the least change in optical properties upon annealing. We associate that with the high melting point of ZrN compared to that of Ag, Al, and Au, as shown in Table S1.

| metal             | Ag   | Al  | Au   | ZrN  |
|-------------------|------|-----|------|------|
| melting point (K) | 1115 | 933 | 1333 | 3225 |
| reference         | [1]  | [2] | [3]  | [4]  |

Table S1: Melting points (K) of the investigated metals

## 2 Characterization

Figure S2 a shows the relationship between the recorded deposition time and the thickness as measured by RBS. Figure S2 b displays the wavelength of minimum reflectance of the MoS<sub>2</sub> films on ZrN shown in Figure 1 against their thickness. The slope of the fitted linear functions is 6.5 and 7.5 for the as-deposited and annealed samples, respectively, indicating that changes in thickness down to one molecular layer ( $\delta=0.65$  nm) could be sensed. The smallest difference between the wavelength of the absorbing states (i.e., reflectance minimum) is 3 nm for the  $\delta = 1.3$  nm sample.

Figure S3 shows the optical properties of the sputtered MoS<sub>2</sub> and ZrN films, together with a comparison with literature values. These are the values used for the Transfer Matrix calculations shown in Figure 1. Given the known thickness dependency of the optical properties in MoS<sub>2</sub>, we report the measured values for different film thicknesses. The presence of ZrN is detrimental to study MoS<sub>2</sub> for several of the characterization techniques used in this work. These include RBS, since molybdenum and zirconium have similar atomic weights and volumes and therefore their characteristic peaks can overlap, 4-point resistance measurements, due to the high conductivity of ZrN, and both Raman and photoluminescence spectroscopies, since the presence of a reflective metal leads to strong background fluorescence. Therefore, MoS<sub>2</sub> is also directly grown on top of a silicon substrate that is capped with 50 nm SiO<sub>2</sub>/50 nm Si<sub>x</sub>N<sub>y</sub>. The deposition and annealing MoS<sub>2</sub> were performed simultaneously independently of the substrate to ensure the same thickness. In contrast to the samples deposited on ZrN, the samples on Si<sub>x</sub>N<sub>y</sub> do not show any color change after annealing and only a very moderate change with increasing MoS<sub>2</sub> thickness, as shown in Figure S4. This demonstrates the importance of tailoring substrates when engineering optical properties.

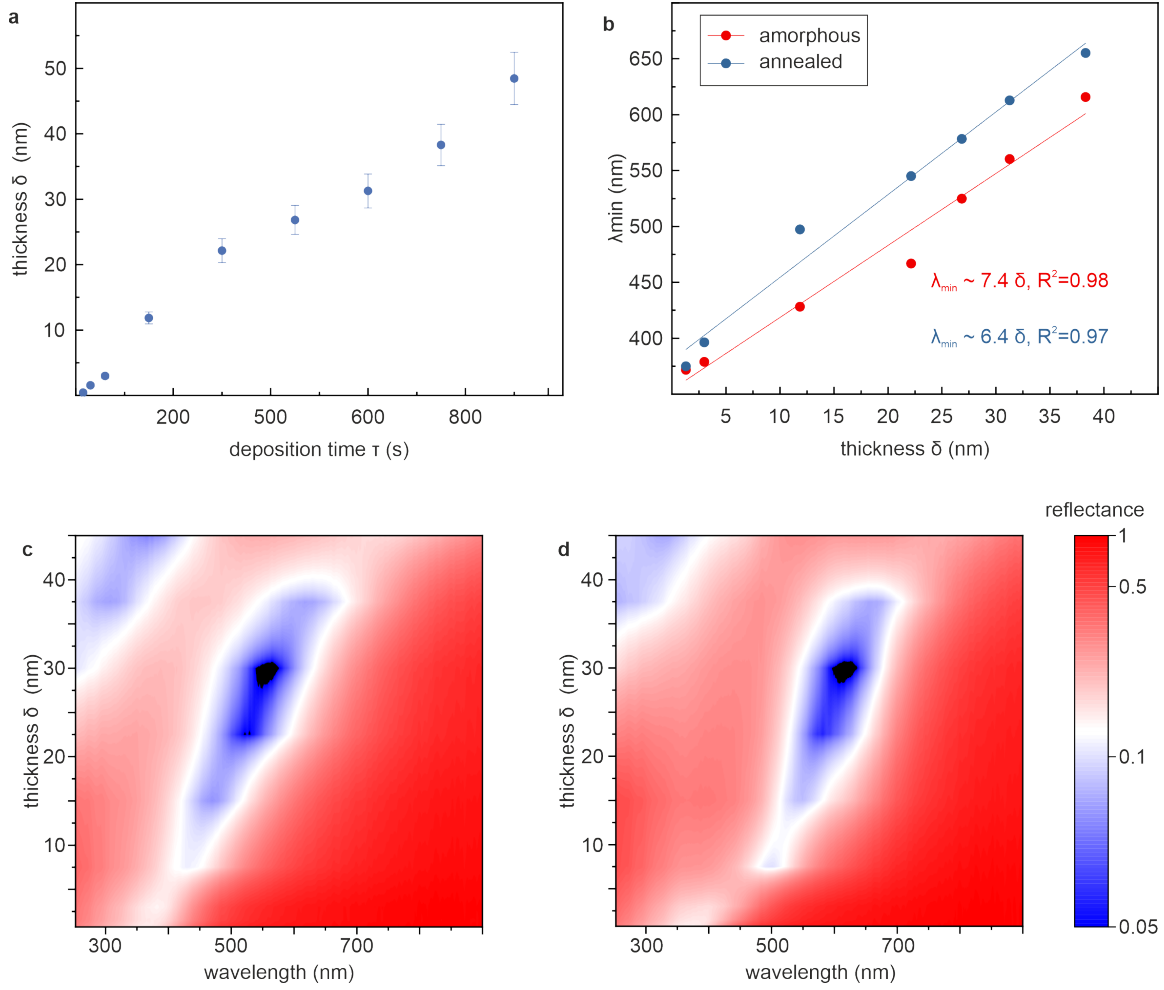

Figure S2: (a): Thickness of the sputtered MoS<sub>2</sub> as measured by RBS films as a function of the deposition time. (b): Wavelength of minimum reflectance against thickness for the thin films of MoS<sub>2</sub> on top of ZrN shown in Figure 1. (c): Color map of the reflectance of aMoS<sub>2</sub> films of different thicknesses. (d): Colormap of the reflectance of cMoS<sub>2</sub> films of different thicknesses.

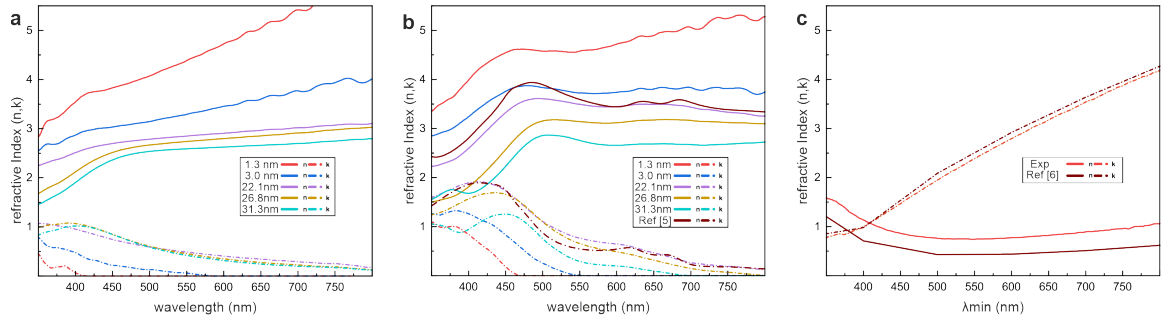

Figure S3: Complex refractive index parameters  $n$  and  $k$  of as measured by ellipsometry of (a): aMoS<sub>2</sub> of different thicknesses, (b): cMoS<sub>2</sub> of different thicknesses and a comparison with literature values [5], and (c): ZrN and a comparison with the literature values [6].

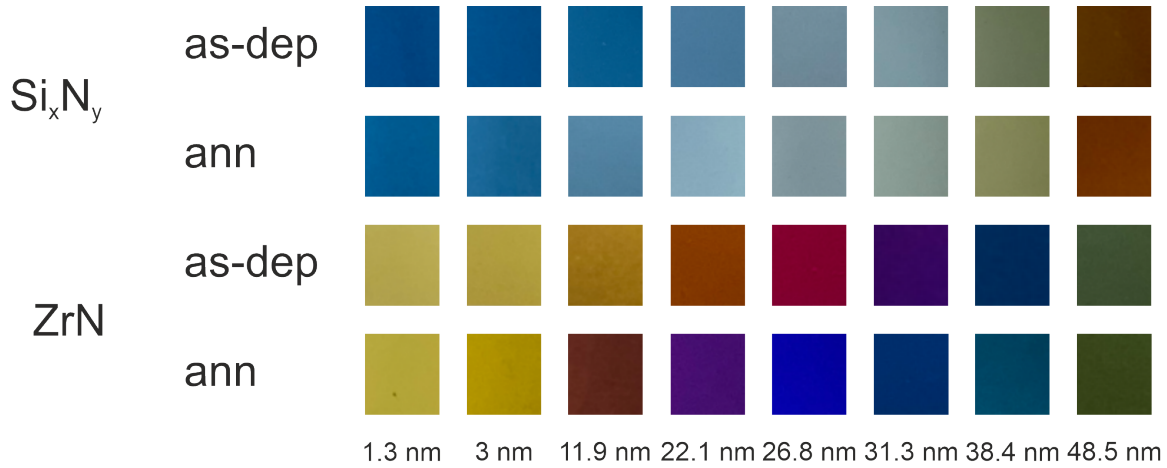

Figure S4: Pictures of samples with different thicknesses of MoS<sub>2</sub> on Si substrates with SixNy (top) and ZrN (bottom) as the last film before MoS<sub>2</sub>.

To assess the thickness of the MoS<sub>2</sub> films using the Raman spectra shown in Fig.2, the peaks were fitted using the following function:

$$y = y_{01} + \frac{A1}{w1 * \sqrt{\frac{\pi}{4 * \ln(2)}}} * e^{-4 * \ln(2) * \frac{(x - x_{c1})^2}{w1^2}} + y_0 + y_{02} + \frac{A2}{w2 * \sqrt{\frac{\pi}{4 * \ln(2)}}} * e^{-4 * \ln(2) * \frac{(x - x_{c2})^2}{w2^2}} \quad (1)$$

Where y<sub>0</sub> is the baseline indicating the background detenction, A1 is the intensity of the peak, x<sub>c</sub> is the central frequency of the peak, and W is the full-width half peak (FWHP). Subscripts 1 and 2 stand for the two different Raman peaks.

Table S2 reports the fit parameters of the characteristic MoS<sub>2</sub> Raman modes shown in Figure 2.

|                      | $\delta=1.3\text{nm}$  |           | $\delta=3\text{nm}$    |           | $\delta=11.9\text{nm}$ |           |
|----------------------|------------------------|-----------|------------------------|-----------|------------------------|-----------|
|                      | Value                  | Std Error | Value                  | Std Error | Value                  | Std Error |
| <b>y0</b> $E_{2g}$   | 0.5041                 | 0.0009    | 1.0261                 | 0.0011    | 1.5066                 | 0.0026    |
| <b>xc</b> $E_{2g}$   | 383.7498               | 0.0506    | 382.9381               | 0.0396    | 380.4773               | 0.0944    |
| <b>w</b> $E_{2g}$    | 3.4034                 | 0.0530    | 4.0297                 | 0.0418    | 4.7229                 | 0.1013    |
| <b>A</b> $E_{2g}$    | 0.2578                 | 0.0034    | 0.4764                 | 0.0041    | 0.4422                 | 0.0079    |
| <b>FWHM</b> $E_{2g}$ | 8.0144                 | 0.1247    | 9.4892                 | 0.0984    | 11.1215                | 0.2385    |
| <b>Area</b> $E_{2g}$ | 2.1995                 | 0.0323    | 4.8122                 | 0.0476    | 5.2347                 | 0.1104    |
| <b>y0</b> $A_{1g}$   | 0.5041                 | 0.0009    | 1.0261                 | 0.0011    | 1.5066                 | 0.0026    |
| <b>xc</b> $A_{1g}$   | 406.9188               | 0.0151    | 406.8657               | 0.0184    | 407.3953               | 0.0447    |
| <b>w</b> $A_{1g}$    | 4.5538                 | 0.0161    | 3.8452                 | 0.0194    | 5.3414                 | 0.0485    |
| <b>A</b> $A_{1g}$    | 0.9954                 | 0.0029    | 0.9993                 | 0.0042    | 0.9887                 | 0.0074    |
| <b>FWHM</b> $A_{1g}$ | 10.7234                | 0.0378    | 9.0547                 | 0.0456    | 12.5780                | 0.1141    |
| <b>Area</b> $A_{1g}$ | 11.3618                | 0.0387    | 9.6316                 | 0.0461    | 13.2376                | 0.1197    |
| <b>R<sup>2</sup></b> | 0.9991                 |           | 0.9983                 |           | 0.9940                 |           |
|                      | $\delta=22.1\text{nm}$ |           | $\delta=26.8\text{nm}$ |           | $\delta=31.3\text{nm}$ |           |
|                      | Value                  | Std Error | Value                  | Std Error | Value                  | Std Error |
| <b>y0</b> $E_{2g}$   | 2.0065                 | 0.0025    | 2.5053                 | 0.0029    | 3.0106                 | 0.0029    |
| <b>xc</b> $E_{2g}$   | 380.1515               | 0.0827    | 380.0081               | 0.1116    | 380.1721               | 0.1166    |
| <b>w</b> $E_{2g}$    | 5.3148                 | 0.0896    | 4.8597                 | 0.1201    | 4.7932                 | 0.1253    |
| <b>A</b> $E_{2g}$    | 0.5092                 | 0.0071    | 0.4215                 | 0.0087    | 0.4083                 | 0.0089    |
| <b>FWHM</b> $E_{2g}$ | 12.5154                | 0.2109    | 11.4437                | 0.2828    | 11.2872                | 0.2951    |
| <b>Area</b> $E_{1g}$ | 6.7836                 | 0.1140    | 5.1347                 | 0.1254    | 4.9058                 | 0.1265    |
| <b>y0</b> $A_{1g}$   | 2.0065                 | 0.0025    | 2.5053                 | 0.0029    | 3.0106                 | 0.0029    |
| <b>xc</b> $A_{1g}$   | 407.3134               | 0.0407    | 407.2793               | 0.0501    | 407.4679               | 0.0515    |
| <b>w</b> $A_{1g}$    | 4.9398                 | 0.0438    | 5.3456                 | 0.0543    | 5.3935                 | 0.0559    |
| <b>A</b> $A_{1g}$    | 0.9949                 | 0.0073    | 0.9816                 | 0.0083    | 0.9760                 | 0.0084    |
| <b>FWHM</b> $A_{1g}$ | 11.6324                | 0.1031    | 12.5880                | 0.1279    | 12.7006                | 0.1317    |
| <b>Area</b> $A_{1g}$ | 12.3189                | 0.1081    | 13.1528                | 0.1335    | 13.1943                | 0.1368    |
| <b>R<sup>2</sup></b> | 0.9946                 |           | 0.9924                 |           | 0.9921                 |           |

Table S2: Fit parameters from the Raman spectra of the annealed MoS<sub>2</sub> on SixNy samples shown in Figure 2 d

We used transmission electron microscopy (TEM) to gain a better understanding of the morphology of the thinnest MoS<sub>2</sub> films. MoS<sub>2</sub> was directly sputtered on Si<sub>3</sub>N<sub>4</sub> grids for 30 s. This type of grid was chosen for its stability during UHV annealing at 485°C. Based on the sputtering time versus thickness as measured by RBS shown in Figure S2, we expect a film thickness of 1.3 nm. Figure S5 summarizes the findings of that investigation.

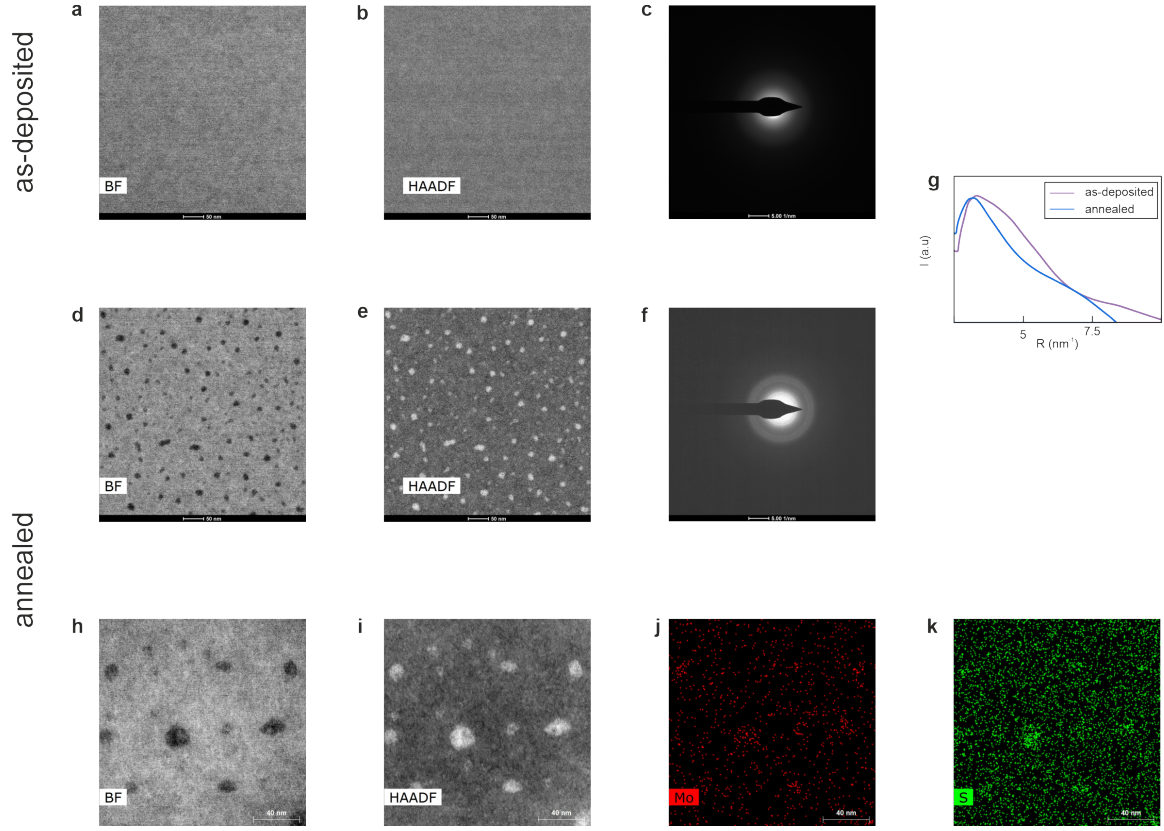

Figure S5: TEM images of MoS<sub>2</sub> films sputtered on a TEM grid for 30s. (a,d,h): Bright-field micrographs of the (a) as-deposited and (d,h) annealed samples. (b,e,i): High-angle annular dark-field micrographs of the (b) as-deposited and (e,i) annealed samples. (c,f): Diffraction patterns of the (c) as-deposited and (f) annealed samples. (g): Comparison between the radial distributions of the diffraction patterns. (j,k): Energy dispersive X-ray spectroscopy results showing the (j) molybdenum and (k) sulfur content of the area of the annealed sample shown in (h-i).

The TEM images of the amorphous sample show no features, indicating uniformity in the

thickness. The diffraction spectrum confirms that the film is amorphous (Figure S5 c). Some small features emerge through crystallization, as shown in Figure SS5 f and g. The Energy Dispersive X-ray spectroscopy (EDX) results (Figure S5 j,k) seem to indicate that the islands have a higher concentration of both S and Mo.

The photoluminescence spectra were fitted with the following function:

$$a1 * e^{-\frac{x-b1}{c1}} + a2 * e^{-\frac{x-b2}{c2}} + a3 * e^{-\frac{x-b3}{c3}} \quad (2)$$

Where a is the intensity of the curve, b is the central wavelength of the peaks, and c is the FWHM. Subscripts 1, 2, and 3 represent the different excitonic peaks. Table 2 reports the fitting parameters that were obtained through peak deconvolution.

|                      | $\delta=1.3\text{nm}$ | $\delta=3\text{nm}$ | $\delta=11.9\text{nm}$ | $\delta=22.1\text{nm}$ | $\delta=31.3\text{nm}$ |
|----------------------|-----------------------|---------------------|------------------------|------------------------|------------------------|
| <b>a1</b>            | 1261.271              | 919.3               | 432.1557               | 409.8988               | 330.786                |
| <b>b1</b>            | 1.778044              | 1.777102            | 1.767949               | 1.771151               | 1.770257               |
| <b>c1</b>            | 0.088672              | 0.087159            | 0.079035               | 0.083499               | 0.077914               |
| <b>a2</b>            | 3166.597              | 2153.129            | 721.9827               | 286.6948               | 193.8602               |
| <b>b2</b>            | 1.941611              | 1.941959            | 1.935478               | 1.927423               | 1.925152               |
| <b>c2</b>            | 0.147327              | 0.145838            | 0.147783               | 0.097779               | 0.08659                |
| <b>a3</b>            | 3986.06               | 3151.53             | 1056.47                | 647.83                 | 423.50                 |
| <b>b3</b>            | 1.24732               | 1.24734             | 1.24855                | 1.25035                | 1.25138                |
| <b>c3</b>            | 0.06914               | 0.06926             | 0.07157                | 0.07492                | 0.07804                |
| <b>R<sup>2</sup></b> | 0.995819              | 0.994765            | 0.979755               | 0.943456               | 0.925294               |

Table S3: Fit parameters of the photoluminescence spectra shown in Figure 2 i.

Figure S6 shows the raw data of the photoluminescence measurements shown in Figure 2 i, together with an example of the fit of a spectrum.

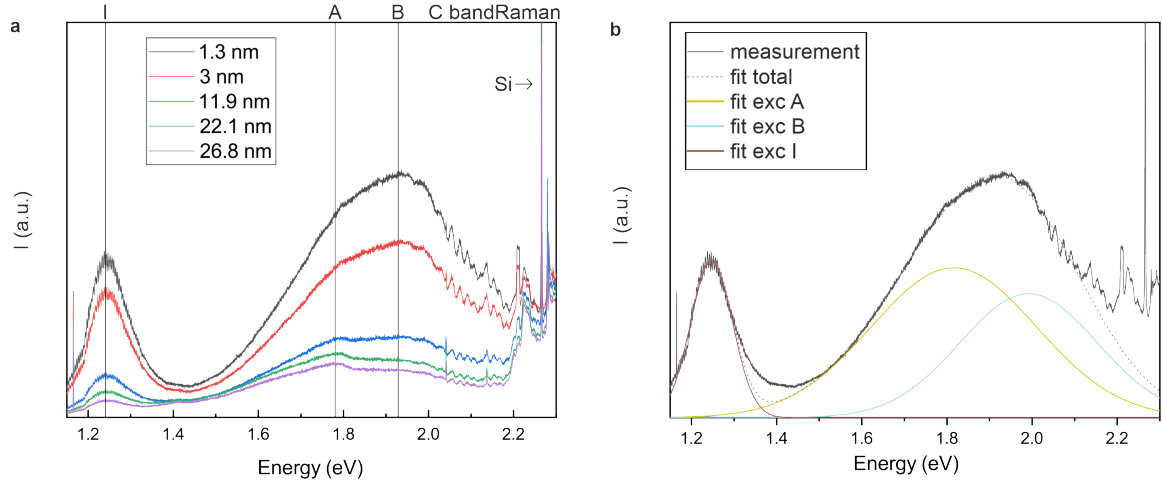

Figure S6: (a): Photoluminescence spectra of cMoS<sub>2</sub> of different thicknesses, analogous to the measurements shown in Figure 2 i. (b): Photoluminescence spectra of cMoS<sub>2</sub> with  $\delta=1.3$  nm together with its fit using the parameters shown in Table 2.

In order to approximate crystallite size using the [002] X-ray diffraction spectra shown in Figure 2, the peaks were fitted using the following function:

$$y = y_0 + \frac{A}{w * \sqrt{\frac{\pi}{4 * \ln(2)}}} * e^{-4 * \ln(2) * \frac{(x - x_c)^2}{w^2}} \quad (3)$$

Where  $y_0$  is the baseline,  $A$  is the intensity of the peak,  $x_c$  is the central frequency of the peak, and  $w$  is the full-width half peak (FWHP).

Table 2 reports the fit parameters of the [002] XRD peaks shown in Figure 2.

|                      | $\delta=31.26\text{nm}$ |                | $\delta=48.45\text{nm}$ |                | $\delta=75.55\text{nm}$ |                |
|----------------------|-------------------------|----------------|-------------------------|----------------|-------------------------|----------------|
|                      | Value                   | Standard Error | Value                   | Standard Error | Value                   | Standard Error |
| <b>y0</b>            | 2493.297                | 63.83753       | 2626.02                 | 40.22401       | 2687.53                 | 39.75144       |
| <b>xc</b>            | 13.80217                | 0.00876        | 13.83436                | 0.00726        | 13.8497                 | 0.0081         |
| <b>A</b>             | 1642.555                | 204.8152       | 1511.53                 | 122.3772       | 1446.063                | 118.6436       |
| <b>w</b>             | 1.6652                  | 0.10403        | 1.53417                 | 0.06632        | 1.48694                 | 0.06689        |
| <b>R<sup>2</sup></b> | 0.93023                 |                | 0.95298                 |                | 0.94296                 |                |

Table S4: Fit parameters of the [002] peak of the XRD spectra of Figure 2 d.

The crystalline size was approximated using the Scherrer equation:

$$\tau = \frac{\lambda}{\beta * \cos\omega} \quad (4)$$

Where  $\tau$  is the crystallite size,  $\lambda$  is the wavelength of the X-ray,  $\beta$  is the width of the diffraction peak, and  $\omega$  is the angular position of the peak. Instrumental broadening was not considered in this approximation, so our calculation slightly underestimates the grain size.

### 3 Smart sensing of the functional properties

Modified hyperbolic functions were used to fit the change in the functional properties of the thin films and the multilayer:

$$y = A \tanh(B(T - T_c)) + D \quad (5)$$

Where B is the slope, T is the annealing temperature of a sample, T<sub>c</sub> is the temperature at which the transition happens, and A and D are geometrical parameters. Table S5 reports the fit parameters.

|                  |                         | <b>A</b>   | <b>B</b> | <b>T<sub>c</sub></b> | <b>D</b>   | <b>R<sup>2</sup></b> |
|------------------|-------------------------|------------|----------|----------------------|------------|----------------------|
| <b>δ=31.26nm</b> | Reflectance Temperature | 0.578      | 0.006    | 494.576              | 0.468      | 0.994                |
|                  | Error                   | 0.121      | 0.002    | 27.229               | 0.065      |                      |
|                  | Resistance Temperature  | 586648.423 | 0.121    | 507.676              | 805838.703 | 0.952                |
|                  | Error                   | 235388.447 | 0.000    | 89.232               | 235398.412 |                      |
| <b>δ=48.45nm</b> | Reflectance Temperature | 0.473      | 0.050    | 515.381              | 0.501      | 0.997                |
|                  | Error                   | 0.035      | 0.394    | 72.070               | 0.032      |                      |
|                  | Resistance Temperature  | 616798.224 | 0.142    | 462.754              | 818368.180 | 0.999                |
|                  | Error                   | 14796.742  | 0.000    | 0.810                | 14796.742  |                      |
|                  | Hardness Temperature    | 0.264      | -0.013   | 579.329              | 1.113      | 0.983                |
|                  | Error                   | 0.048      | 0.005    | 19.313               | 0.042      |                      |
| <b>δ=75.55nm</b> | Reflectance Temperature | 0.491      | 0.017    | 485.854              | 0.492      | 0.997                |
|                  | Error                   | 0.032      | 0.003    | 8.192                | 0.031      |                      |
|                  | Resistance Temperature  | 603790.113 | 0.099    | 462.698              | 694784.693 | 1.00                 |
|                  | Error                   | 62795.073  | 0.000    | 1.497                | 62795.106  |                      |
|                  | Hardness Temperature    | 0.173      | -0.037   | 594.292              | 1.033      | 0.845                |
|                  | Error                   | 0.086      | 0.655    | 103.035              | 0.086      |                      |

Table S5: Fit parameters of the changes of the functional properties of MoS<sub>2</sub> thin films shown in Figure 3.

Based on Table S5, the estimated transition temperature taking into account all three techniques is 521±171 K. The mechanical characterization leads to a higher crystallization temperature and has the highest error. The transition temperature between the two states is 499±79 K, 478±93 K, and 587±105 K when only the results of the optical, electrical, and mechanical

characterization are considered, respectively.

The resistance of the samples shown in Figure 1 is also characterized in order to confirm the increase in the sheet resistance upon annealing at 750K for two hours. Figure S7 shows the results of the 4-point measurements.

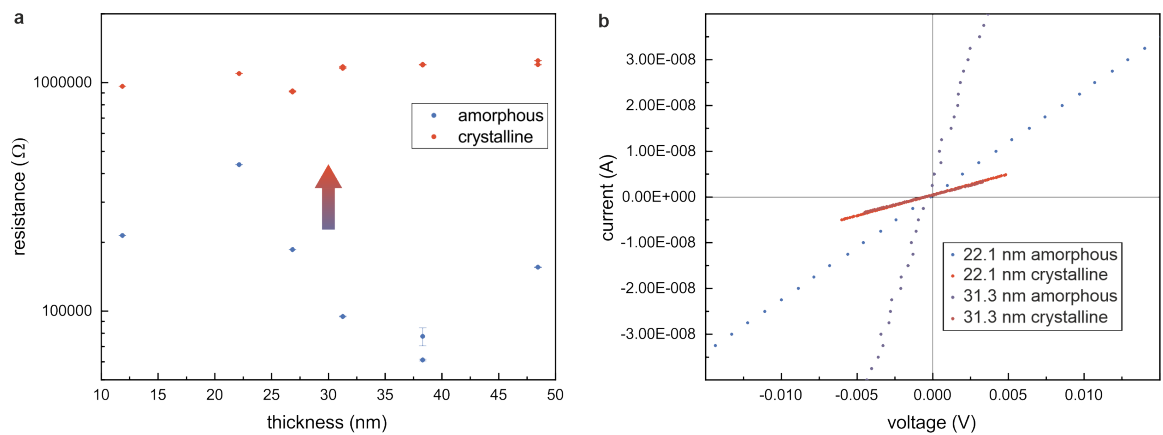

Figure S7: (a): Change in the sheet resistance upon annealing for  $\text{MoS}_2$  films with different thickness. The amorphous samples were as-deposited, while the crystalline samples were annealed at 750K. (b): I-V curves of two selected  $\text{MoS}_2$  thicknesses before and after annealing at 750K.

## 4 Few-layer MoS<sub>2</sub> multilayer composites

To elaborate on the correlation between the different functional properties of the multilayer, we plot the relationship between the hardness and the wavelength of minimum reflection of the multilayer at different temperatures. Figure S8 a shows two clearly differentiated states: one characterized by high hardness and low  $\lambda_{min}$  before annealing and lower hardness and higher  $\lambda_{min}$  after annealing, as discussed in Figure 4.

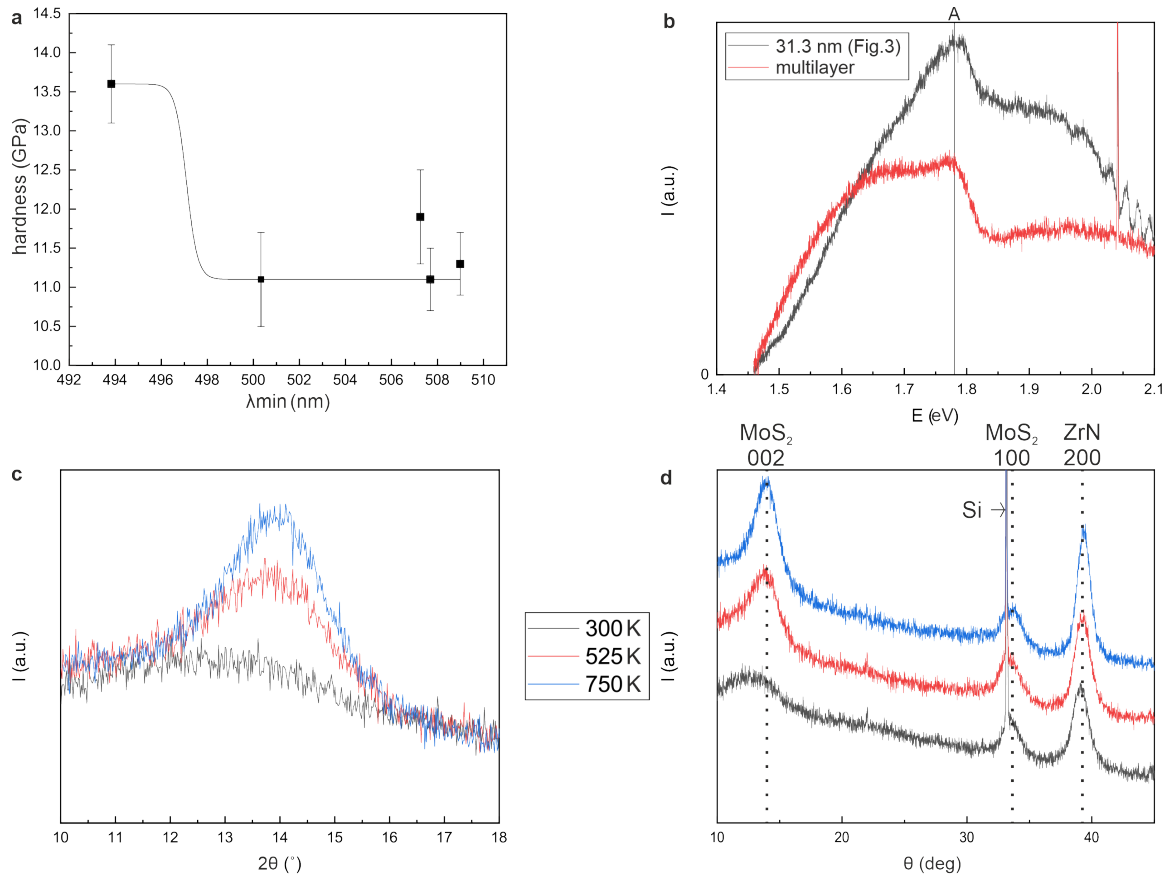

Figure S8: (a): Photoluminescence spectra of the  $\delta=31.26$  nm film shown in Figure 3 and of the multilayer shown in Figure 4. (b): Hardness of the ZrN-MoS<sub>2</sub> multilayer against the wavelength of the minimum in reflectance. (c and d): X-ray diffraction spectra of the multilayer annealed at different temperatures. [7] ICSD(644895) [8] ICSD(31067)

Photoluminescence experiments were also conducted on the multilayer shown in Figure 4,

composed of three stacked 12 nm ZrN-13 nm MoS<sub>2</sub> bilayers. The results are shown in Figure S8 together with the photoluminescence spectra of a sample with a similar MoS<sub>2</sub> nominal thickness. The A excitonic peak can be observed in the multilayer sample, proving that ZrN/MoS<sub>2</sub> multilayers support photoluminescent modes. Figure S8 c and d show the X-ray diffraction results of the multilayer after different annealing temperatures. The results confirm that the change in optical and mechanical properties upon annealing is due to crystallization.

When looking at composites or multilayer materials, the rule of mixtures provides a model for predicting expected mechanical behavior through a linear combination of component materials' properties that are scaled by their relative volume fractions. For the MoS<sub>2</sub>/ZrN multilayer system, the effective hardness of the multilayer ( $H_{ml}$ ) can be defined as [9, 10]:

$$H_{ml} = V_{ZrN} \cdot H_{ZrN} + (1 - V_{ZrN}) \cdot H_{MoS_2} \quad (6)$$

where  $H_{ZrN}$  and  $H_{MoS_2}$  are the hardness of ZrN and MoS<sub>2</sub>, respectively, and  $V_{ZrN}$  the ZrN volume fraction.

## References

- [1] Sharma, R. C. and Chang, Y. A., *Bulletin of Alloy Phase Diagrams* **1986**.
- [2] Sharma, R. C. and Chang, Y. A., *Journal of Phase Equilibria* **1987**.
- [3] Okamoto, H. and Massalski, T. B., *Bulletin of Alloy Phase Diagrams* **1985**.
- [4] Gribaudo, L. and Arias, D. and Abriata, J., *Journal of Phase Equilibria* **1994**.
- [5] Islam, Kazi M., Synowicki, Ron, Ismael, Timothy, Oguntoye, Isaac, Grinalds, Nathan, Escarra, Matthew D., *Advanced Photonics Research* **2021**.
- [6] Ribbing, Carl G. and Roos, Arne, *Handbook of Optical Constants of Solids* **1997**.
- [7] Hassel, O., *Zeitschrift fr Kristallographie* **1924**.
- [8] Constant, K., Kieffer, R., Ettmayer, P., *Monatshefte fr Chemie* **1975**.
- [9] Falk, Michael L. and Langer, J.S, *Annual Review of Condensed Matter Physics* **2011**.
- [10] Wang, H. F., Yang, X., Bangert, H., Torzicky, P., Wen, L., *Thin Solid Films* **1992**.
